# Supplementary material for: Helicity conservation by flow across scales in reconnecting vortex links and knots
Source: arXiv:1404.6513 ancillary file (2014-09-18)
Supplement: Supplementary file 1 [file supplemental.pdf]

# Helicity conservation in topology-changing reconnections: the flow of linking and coiling across scales – Supplemental Materials

Martin W. Scheeler,<sup>1,\*</sup> Dustin Kleckner<sup>\*,1,†</sup> Davide Proment,<sup>2</sup> Gordon L. Kindlmann,<sup>3</sup> and William T.M. Irvine<sup>1,‡</sup>

<sup>1</sup>*James Franck Institute, Department of Physics,  
The University of Chicago, Chicago, Illinois 60637, USA.*

<sup>2</sup>*School of Mathematics, The University of East Anglia, NR4 7TJ Norwich, Norfolk, UK.*

<sup>3</sup>*Computation Institute, Department of Computer Science,  
The University of Chicago, Chicago, Illinois 60637, USA.*

## Experimental vortex generation

The experiments were carried out using the vortex-generation and imaging techniques described in [1]. Vortices are generated using shaped hydrofoils generated by a 3D printer. These hydrofoils are attached to a frame which is then rapidly accelerated using a short, open pneumatic cylinder driven by a quick-release valve, where typical accelerations are on the order of  $a = 285 \text{ m/s}^2$ , reaching speeds of  $U \sim 2 \text{ m/s}$ . The hydrofoils used for the data shown in the main text have a chord of  $Ch = 22.5 \text{ mm}$ , a leading edge thickness of  $t_1 = 3.75 \text{ mm}$ , a trailing edge thickness of  $t_2 = 0.225 \text{ mm}$ , and a bend of  $\theta = 15^\circ$ . Images of the 3D models used to print each hydrofoil are reproduced in Figure S1.

The trailing edge path (which is traced by the resulting vortices) had an r.m.s. radius of  $\bar{r} = 69.3 \text{ mm}$  in the case of the trefoil knot and an r.m.s. radius of  $\bar{r} = 75.5 \text{ mm}$  in the case of the linked rings. Hydrofoils (and vortices) have also been generated at smaller scales, and are observed to have qualitatively similar dynamics. A volumetric image of the vortex core is obtained with a laser-scanning tomography apparatus (the obtained volumes have a size of  $384^3$  voxels with an adjustable resolution of  $0.6 \text{ mm/voxel}$ ). The effects of perspective in the imaging apparatus are corrected for in the resulting

data. The circulation of the vortices is estimated using the formula for the circulation around a thin flat plate in inviscid flow [2]:

$$\Gamma = \pi U Ch \sin \alpha, \quad (1)$$

where  $\alpha \approx \theta/2$  is the effective angle of attack. The speed of the hydrofoil is directly measured using an encoder attached to the hydrofoil acceleration frame. The circulation obtained from this estimate is consistent with the forward speed of simple vortex rings and the stretching rate observed for knotted vortices.

## Experimental vortex shape reconstruction

To reconstruct the shape of the vortices from experimental volumetric data, we have adapted methods from biomedical image analysis. Due to the nature of the raw data, some apparent gaps along the vortex path may arise from non-uniform bubble density. Previously, manual identification of vortices was used, along with automated line tracing [1]. As an improvement, we have developed a two-step process for numerically identifying vortices before joining them together into a complete path.

Vortices appear as one-dimensional ridge lines in the three-dimensional image: the locus of points for which image intensity is maximized relative to motion along the minor and medium eigenvectors of the image Hessian [3]. For the detection and spatial localization of vortices we adapt a method of particle-based ridge sampling [4]. Image identification ‘particles’ move within the image domain, subject to forces from other particles, while constrained to stay within ridge lines. These particles are subject to a synthetic radial potential function that monotonically decreases away from  $r = 0$  but with a slight attractive potential well at tunable position, producing approximately equi-distant spacing. The point locations are iteratively updated to minimize the total energy of the system. Point are periodically added to ensure complete coverage of detected ridge features, and deleted where the feature fades to noise. For each energy minimizing iteration, the points are constrained to ridges with Newton optimization using the gradient and Hessian of the continuous image, as reconstructed by convolution with the  $C^2$  cubic B-spline.

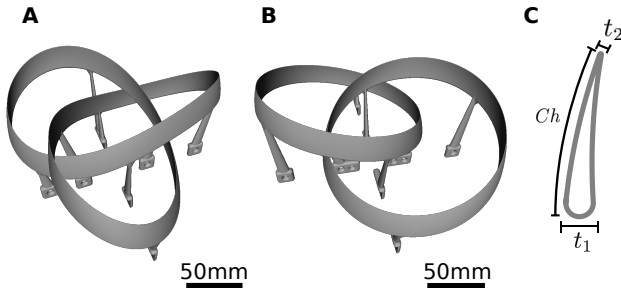

FIG. S1: (A) A 3D rendering of the trefoil knot hydrofoil used in experiment. (B) A 3D rendering of the link rings hydrofoil used in experiment. (C) The hydrofoil cross-section used in both the trefoil knot and linked rings with the following specifications: a chord of  $Ch = 22.5 \text{ mm}$ , a leading edge thickness of  $t_1 = 3.75 \text{ mm}$ , a trailing edge thickness of  $t_2 = 0.225 \text{ mm}$ , and a bend of  $\theta = 15^\circ$ .

Once particles have converged, the recovered vortex segments are joined via fast marching [5].

### Gross-Pitaevskii equation

Simulations of the Gross-Pitaevskii Equation (GPE) were carried out using the same parameters as in [6], where the GPE is considered in a de-dimensionalized form:

$$2i\partial_t\Psi + \nabla^2\Psi - |\Psi|^2\Psi = 0, \quad (2)$$

where the circulation in these units is  $\Gamma = 2\pi$ , the healing length is  $\xi = 1$ , and the far-field density is  $\rho_\infty = |\Psi_\infty|^2 = 1$ . The simulations employed a grid size of  $\Delta x = \xi/2$  and time-step  $\Delta t = 0.02$ , using periodic boundary conditions. The initial phase field was constructed by brute-force integration of the velocity field generated by the vortices (obtained from the Biot-Savart law), making use of the relation:

$$\phi_{\mathbf{x}_1} - \phi_{\mathbf{x}_0} = \int_{\mathbf{x}_0}^{\mathbf{x}_1} \mathbf{v} \cdot d\boldsymbol{\ell}, \quad (3)$$

where the periodicity is ensured by calculating the flow field for periodically copied versions of the desired vortex. (In practice, we employ a  $5 \times 5 \times 5$  cube of vortex copies, where the flow field is calculated in the central volume; this number was chosen empirically to produce smooth boundaries that do not generate sound waves when the simulation begins.) A similar integration method has recently been employed for GPE simulations in other contexts [7]. To create a phase volume, an arbitrary phase is assigned to one corner, which is then extended to a plane on one edge of the volume. Integrating from this plane then produces a phase volume. To ensure that the phase matches across periodic boundaries, a constant gradient is added. (This is equivalent to removing the uniform background flow produced by a periodic collection of vortex loops.)

The initial density field was calculated using a Padé approximant [8]:

$$\rho(r) = \frac{\frac{11}{32}r^2 + \frac{11}{384}r^4}{1 + \frac{1}{3}r^2 + \frac{11}{384}r^4}, \quad (4)$$

where  $r$  was taken to be the distance to the closest vortex line. The vortex knot with r.m.s. radius  $\bar{r} = 24\xi$  was simulated in a periodic cube with edge  $a = 128\xi$  (256 grid points), and the simulation volume was scaled in proportion to the knots for other sizes. Weak density waves are observed to radiate from the vortex at the beginning of the simulation (due to the fact that the vortex curvature relaxes the core profile to a slightly different form than that given by the Padé approximant), resulting in a small reduction of the vortex length and energy from the

initial condition. Vortex paths were obtained by tracing the phase defects in the simulated wave function. Time-steps when the vortices begin to overlap, defined as when the vortex separation is less than  $r_{min} < 2\xi$ , are omitted from Fig. 4.

### Calculation of linking and writhe

Linking and writhe are computed by projecting the three-dimensional paths into a plane and counting signed crossings between line segments. To protect against numerical errors, which may be especially problematic with the noisy experimental data, three random orientations are checked for consistency, and more orientations are computed if the results do not agree. To compute the non-integer portion of the writhe, an additional term is added to account for the twist of the implied framing [9]. A black-board framing (i.e. a framing chosen to always be exactly perpendicular to the projection direction) is used instead of the traditional Frenet-Serret framing; this was found to produce more accurate results in the presence of noise, as confirmed by comparing the results to the average summed crossing number over random projections.

### Biot-Savart evolution of thin core vortices

The Biot-Savart velocity of the vortex is calculated using an exact expression for the flow generated by non-adjacent segments (modeled as a polygonal path), and an explicit expression for the flow generated by the neighboring segments (treated as a circular arc going through the 3 point neighborhood). Time-integration is performed using a 5th order Runge-Kutta scheme (Dormand-Prince [10]) with an adaptive time step so that the velocity error is kept below  $\delta v \lesssim 10^{-10} \Gamma/r_0$  (with segment length  $\Delta\ell \sim 0.05$ ).

### Definition of the centerline helicity

In defining the ‘centerline helicity’, we are forced to adopt a convention for the implied contribution of the twist component of the total helicity. Physically, this corresponds to making a choice for how the vortex bundle should be wrapped around the centerline when twist can not be directly resolved (Fig. S2). Our definition corresponds to the total helicity of a bundle with particularly simple internal structure, so that the total twist component is zero,  $Tw_i = 0$ , resulting in:

$$\mathcal{H}_c \equiv \mathcal{H}_{c, \text{p.t.}} = \Gamma^2 \left( \sum_{i \neq j} \mathcal{L}_{ij} + \sum_i Wr_i \right). \quad (5)$$

Such a result can be obtained by constructing a bundle using the ‘parallel transport’ framing, defined as one for which the twist rate of the normal vector,  $\hat{\mathbf{n}}$ , is everywhere zero:  $(\hat{\mathbf{n}} \times \partial_s \hat{\mathbf{n}}) \cdot d\ell = 0$ .

To illustrate the consequences of our convention, consider a helix defined by:

$$x = a \cos kz \quad (6)$$

$$y = a \sin kz \quad (7)$$

For a section spanning  $z = 0$  to  $z = L$ , the number of helical turns is  $N = \frac{kL}{2\pi}$  and the writhe is:

$$Wr = N(1 - \cos \theta), \quad (8)$$

where the winding angle is  $\theta = \tan^{-1} ka$ . In the limit of small winding angle ( $\theta \rightarrow 0$ ), the resulting helicity is then given by:

$$\mathcal{H}_{c, \text{p.t.}} = \Gamma^2 Wr \quad (9)$$

$$\sim \Gamma^2 \frac{N\theta^2}{2}. \quad (10)$$

This has the important property that helicity goes smoothly to zero as the helix is flattened into a straight line. One apparent disadvantage of the parallel transport framing is that, in general, it does not close, meaning that an individual vortex filament does not reconnect with itself in a single trip around the bundle. We note, however, that this is expected for continuum fields; so long as a local twist rate can be defined, a non-integer total twist can be computed and corresponds to the mean linking of vortex filaments in the bundle [11].

One way to resolve the non-closure of the bundle is to use a Frenet-Serret basis (in other words,  $\hat{\mathbf{n}}$  is the Frenet-Serret normal vector). In this case, the twist and helicity are given by:

$$Tw_{f.s.} = \frac{1}{2\pi} \int ds \tau = N \cos \theta \quad (11)$$

$$\mathcal{H}_{c, f.s.} = \Gamma^2 (Wr + Tw_{f.s.}) = \Gamma^2 N. \quad (12)$$

Note that this result always gives an integer ( $n\Gamma^2$ ) helicity, which is independent of the winding angle. Plotting the bundle resulting from such a framing reveals the source of this extra helicity: the vortex filaments become significantly twisted as the winding angle is reduced (Fig. S2, left side). In fact, integer helicity always result for framings in which all filaments close with themselves, as they produce a uniform, integer filament linking. Furthermore, it follows that the helicity computed for such a bundle will change discontinuously under smooth deformations, as it is confined to integer values. This is especially problematic when computing the helicity for experimental data: even infinitesimal spirals will appear to have high helicity content, and so this convention produces wildly fluctuating centerline helicity. (In the context of the Frenet-Serret framing, this can also be viewed

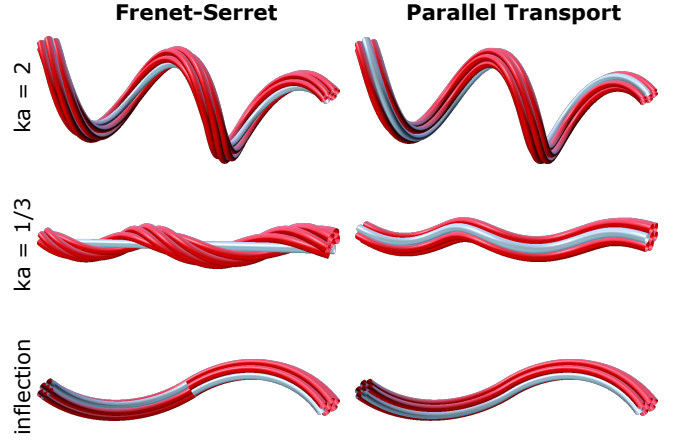

FIG. S2: An illustration of the vortex bundles produced for spiral-like centerlines using different framing methods. The left column shows bundles oriented with the Frenet-Serret normal vector, while the right uses a parallel transport (untwisted) framing. The first two rows are helices, while the third row shows an inflection point produced by merging two circular arcs.

as due to the creation of inflection points, which cause the torsion to be undefined [12]).

In addition to its ease of computation, the centerline helicity for a parallel transport bundle has one other important property: it corresponds to the configuration that naturally results from viscous dissipation of the vortex core (as derived in the next section for a straight centerline). Moreover, our experimental results indicate that it is continuous through a vortex reconnection, suggesting it is the natural and relevant definition for helicity conservation.

### Helicity dissipation for a twisted core

Consider a straight centerline, uniformly twisted core vortex with profile:

$$\boldsymbol{\omega} = \Omega(r) \left( \hat{\mathbf{z}} + r\tau \hat{\boldsymbol{\phi}} \right), \quad (13)$$

where  $\Omega(r)$  is the scalar core profile and  $\tau$  is the twist rate. The helicity dissipation rate is given by: [13]

$$\partial_t \mathcal{H} = -2\nu \int \boldsymbol{\omega} \cdot (\nabla \times \boldsymbol{\omega}) dV = -4\nu\tau \int \Omega^2(r) dA dz, \quad (14)$$

which can be rewritten as a relative decay rate:

$$\partial_t \mathcal{H} = -\mathcal{H} \frac{8\pi\nu}{A_{eff}}, \quad (15)$$

where  $A_{eff}$  is an effective core area given by:

$$A_{eff} = \frac{(\int \Omega(r) dA)^2}{\int \Omega^2(r) dA}. \quad (16)$$

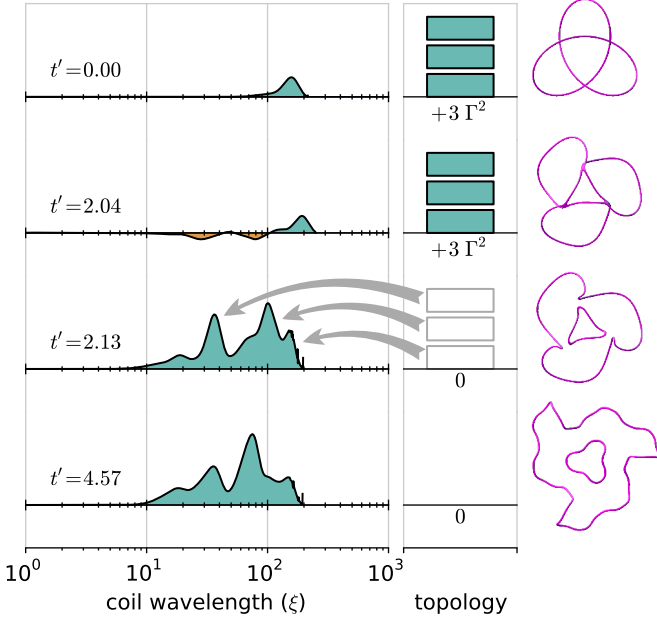

FIG. S3: A helistogram for a GPE trefoil knot with  $\bar{r} = 36\xi$ , shown along with renderings of the density iso-surfaces at the same simulation time. Unlike in the experiments, the perfect symmetry of the simulation causes all three reconnections to happen simultaneously, transferring nearly all of the helicity from knotting to coiling in a single event.

Equivalently, we note that this is equivalent to a dissipation of the total twist:  $\partial_t Tw = -Tw \frac{8\pi\nu}{A_{eff}}$ , where the total twist is given by  $Tw = \int \tau ds$ . For experimental vortices in a viscous fluid, the core size is expected to grow like  $r \sim \sqrt{4\nu t}$ , or  $\sim 2\text{mm}$  for our experiments (for water,  $\nu = 1.0 \text{ mm}^2 \text{ s}^{-1}$  and the typical experimental timescale is  $t \sim 1 \text{ s}$ , which is roughly the time at which the reconnection start). The resulting dissipation rate is:  $\partial_t Tw / Tw \sim 5 \text{ s}^{-1}$ .

### Helistogram analysis

Helistograms for a given curve are constructed by smoothing the original path with a Blackmann windowed sinc kernel of increasingly larger cutoff wavelengths incremented by a small  $d\lambda$ . By taking the difference between the helicity  $\mathcal{H}(\lambda)$  calculated for a path smoothed by  $\lambda$  and the helicity  $\mathcal{H}(\lambda + d\lambda)$  of the slightly more smoothed path, we can compute the helicity stored on the scale of  $\lambda$ . This progressive smoothing process can be seen in supplemental video S1, which shows the path corresponding to each cutoff wavelength.

For a helically wound ring, the locations of the peaks on a helistogram correspond to the helical wavelength  $L/n$  of the path, where  $L$  is the total length of the path and  $n$  is the winding number. A collection of helically wound rings with different values of  $L/n$  along with their

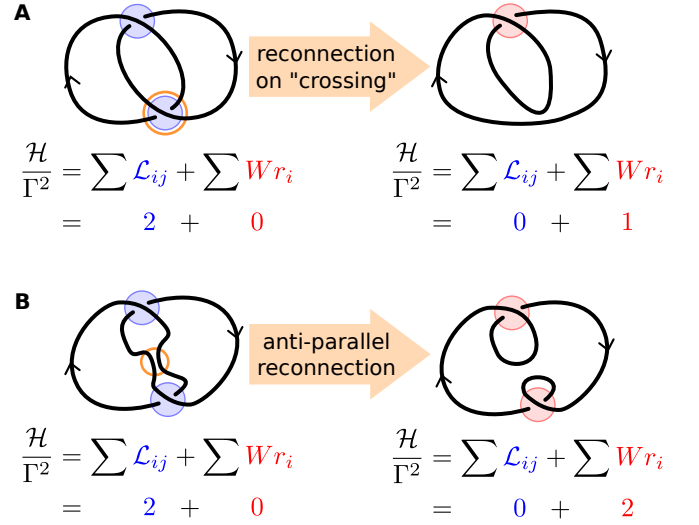

FIG. S4: (A) A diagram of a reconnection event occurring at a 'crossing' for a nearly planar pair of linked rings. The helicity has an apparent change of  $1\Gamma^2$  because an in-plane crossing is eliminated. (B) A reconnection event that occurs between anti-parallel segments does not change the crossing number and so it conserves helicity.

corresponding helistograms are shown in supplemental video S2. Note that as the helical wavelength of the structures increases, the helicity should decrease in magnitude and shift to larger length scales, both of which are captured by the shrinking and translation of the single peak in the helistogram. Helistograms can also be constructed for GPE data, as shown in Fig. S3; the results are qualitatively similar to experimental data for the same initial shape, although all three reconnections happen simultaneously.

### Theory of helicity conservation through a reconnection

As described in the main text, the conservation of helicity in reconnecting vortices is due to the reconnection events happening across regions where the vortex path is anti-parallel. Typically, linking is described in terms of planar knot-diagrams, however, in this case it does not produce an intuitive description of the observed mechanism. For example, vortex reconnections are conventionally depicted as taking place at crossings in a planar diagram (Fig. S4A), leading one to the incorrect conclusion that helicity must change by  $|\Delta\mathcal{H}_c| = 1\Gamma^2$ . (We note that, in all cases, the centerline helicity is given by:  $\mathcal{H}_c/\Gamma^2 = \sum \mathcal{L}_{ij} + \sum Wr_i = N_+ - N_-$ , where  $N_{\pm}$  are the number of signed crossings, averaged over all projections. For nearly planar shapes, all projections have the same number of crossings.) We can modify our diagram to add two-antiparallel extensions, and place the

reconnection in this region; in this case we conclude the helicity is conserved (Fig. S4B). Although this geometry seems unintuitive in a plane, it forms naturally for fully three-dimensional paths. This is particularly true for reconnecting vortices driven by stretching, which are expected to adopt an anti-parallel configuration in order to conserve energy [1]. In the event that the reconnection is not perfectly anti-parallel, as is apparently the case for small GPE vortices, this conservation may be imperfect.

---

\* These two authors contributed equally.

† Electronic address: dkleckner@uchicago.edu

‡ Electronic address: wtmirvine@uchicago.edu

- [1] Kleckner, D. & Irvine, W. T. M. Creation and dynamics of knotted vortices. *Nature Physics* **9**, 253–258 (2013).
- [2] Acheson, D. J. *Elementary Fluid Dynamics* (Clarendon Press, Oxford, 1990).
- [3] Eberly, D. *Ridges in Image and Data Analysis* (Springer, 1996).
- [4] Kindlmann, G. L., Estépar, R. S. J., Smith, S. M. & Westin, C.-F. Sampling and Visualizing Creases with Scale-Space Particles. *IEEE Trans. Visualization and Computer Graphics* **15**, 1415–1424 (2009).
- [5] Sethian, J. A. A fast marching level set method for monotonically advancing fronts. *Proceedings of the National Academy of Sciences of the United States of America* **93**, 1591–5 (1996).
- [6] Proment, D., Onorato, M. & Barenghi, C. Vortex knots in a Bose-Einstein condensate. *Physical Review E* **85**, 1–8 (2012).
- [7] Salman, H. Breathers on Quantized Superfluid Vortices. *Physical Review Letters* **111**, 165301 (2013).
- [8] Berloff, N. G. Padé approximations of solitary wave solutions of the GrossPitaevskii equation. *Journal of Physics A: Mathematical and General* **37**, 1617–1632 (2004).
- [9] Klenin, K. & Langowski, J. Computation of writhe in modeling of supercoiled DNA. *Biopolymers* **54**, 307–17 (2000).
- [10] Dormand, J. & Prince, P. A family of embedded Runge-Kutta formulae. *Journal of Computational and Applied Mathematics* **6**, 19–26 (1980).
- [11] Arnold, V. I. The Asymptotic Hopf Invariant and Its Applications. *Selecta Math. Sov.* **5**, 327 (1986).
- [12] Moffatt, H. & Ricca, R. Helicity and the Calugareanu invariant. *Proceedings of the Royal Society A: Mathematical, Physical and Engineering Sciences* **439**, 411 (1992).
- [13] Moffatt, H. K. Degree of Knottedness of Tangled Vortex Lines. *Journal of Fluid Mechanics* **35**, 117–129 (1969).
